# Supplementary material for: Private Agent-Based Modeling
Source: arXiv:2404.12983 source file (2024-04-19)
Supplement: Supplementary file 1 [file supplementary.tex]

\appendix
\onecolumn

{\color{red} TO BE SUBMITTED SEPARATELY. Maybe fits in the main text}

\section{Calibration experimental details}

To perform GVI as outlined in \autoref{sec:experiment_calibration}, we consider $\mathcal Q$ to be a masked auto-regressive normalizing flow, described by 16 transformations parameterized by 2 hidden layers with 64 hidden units each. We use the \textsc{NormFlows} package \cite{Stimper2023} to implement the flow. $\ell$ is the MMD loss \cite{cherief-abdellatifMMDBayesRobustBayesian2020}. We set the hyperparameter $w=5\cdot 10^{-3}$, and we train using the AdamW \cite{loshchilov2018decoupled} optimizer with a learning rate of $\eta = 10^{-3}$ and a batch size of 10. The whole pipeline is implemented using the \textsc{BlackBirds} \cite{quera-bofarullBlackBIRDSBlackBoxInference2023} library.
